# Supplementary material for: Modeling magnetic evolution and exchange hardening in disordered magnets: The example of Mn$_{1-x}$Fe$_x$Ru$_2$Sn Heusler alloys
Source: arXiv:1910.07543 source file (2019-10-16)
Supplement: Supplementary file 1 [file supporting_info.pdf]

# Supporting Info For: Modeling magnetic evolution and exchange hardening in disordered magnets: The example of $Mn_{1-x}Fe_xRu_2Sn$ Heusler alloys

October 12, 2019

## 0.1 Additional Snapshots

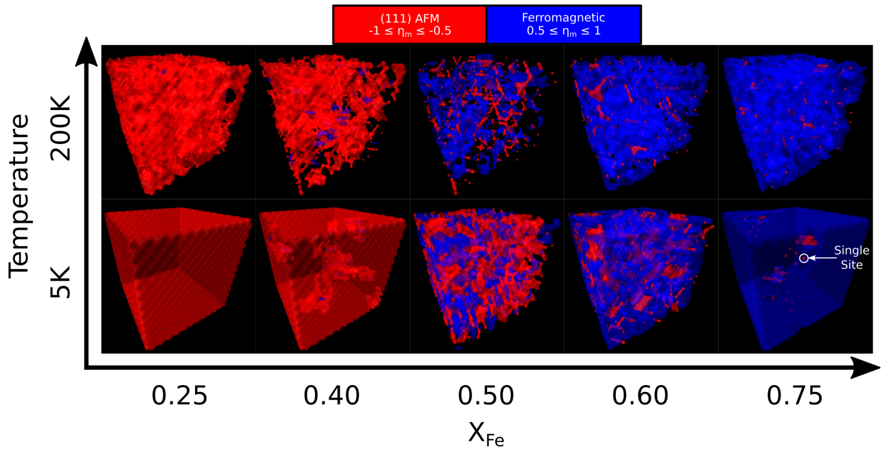


Figure 1: Snapshots of short-range magnetic orderings in chemically-disordered $Mn_{1-x}Fe_xRu_2Sn$ Heuslers colored by local magnetic order parameter, at 5 K and 200 K and at various compositions. All snapshots represent a 12×12×12 tiling of FCC conventional cells. The white circle indicates a single Mn atom that displaying AFM odering with respect to its neighbors.

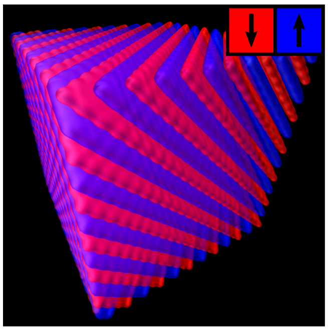

Figure 2: Spin ordering at x=0.25 and T=5 K, demonstrating (111) AFM ordering.

## 0.2 Simulation Details

Properties were averaged between a sufficient number of microstates sampled both after an initial equilibration period and separated in time as to be considered uncorrelated. Fully-equilibrated simulations where performed in a cubic cells containing 4000 primitive cells (8×8×8 box of FCC cells), with temperature steps of ±5K. In the range $T$ = [235, 255]K, in steps of 1K, were performed in a 16×16×16 box of FCC cells, to better resolve the tricritical point.

Chemically-quenched simulations were performed in cubic cells containing 6912 primitive cells ($12\times12\times12$ box of FCC cells).The annealing stage was performed at $T = 1173$ K. 100 snapshots, taken 1000 passes apart, were captured. Each of the 100 high temperature snapshots were chemically frozen, only allowing magnetic degrees of freedom to relax during subsequent cooling runs in 5 K steps. Finally, at each temperature from the cooling stage, the per-snapshot ensemble variables were averaged together to produce approximations of the true ensemble variables.

Our cluster expansion included a magnetic basis function corresponding to a nearest-neighbor tetrahedron of the form $m_i m_j m_k m_l$. This basis function was replaced by $[(\boldsymbol{m}_i \cdot \boldsymbol{m}_j)(\boldsymbol{m}_k \cdot \boldsymbol{m}_l) + (\boldsymbol{m}_i \cdot \boldsymbol{m}_k)(\boldsymbol{m}_j \cdot \boldsymbol{m}_l) + (\boldsymbol{m}_i \cdot \boldsymbol{m}_l)(\boldsymbol{m}_j \cdot \boldsymbol{m}_k)]/3$ since it is equivalent to the tetrahedron basis function for collinear spins and is a suitable first-order approximation when extending an Ising model to a Heisenberg model.[1] Additionally, we introduced three biquadratic terms of the form $(\boldsymbol{m}_i \cdot \boldsymbol{m}_{i'})^2 \times ([1, x_i,$ or $x_i x_j])$ to lift a degeneracy of the AFM ground state.[2, 3]

In our discussion of low-temperature properties, we project the spin vectors onto a common vector to recover a model with Ising-like antiparallel “up” and “down” spins for the purposes of analysis and visualization. At $T = 5$ K, the average magnitude of the dot product between any spin and the common vector is $\geq 0.97$ in all cases.

# Bibliography


[1] R. Drautz and M. Fähnle, Parametrization of the magnetic energy at the atomic level, Phys. Rev. B - Condens. Matter Mater. Phys. **72**, 212405 (2005).

[2] A. L. Wysocki, K. D. Belashchenko, and V. P. Antropov, Consistent model of magnetism in ferropnictides, Nat. Phys. **7**, 485–489 (2011), arXiv:1011.1715 .

[3] S. Khmelevskyi, E. Simon, and L. Szunyogh, Antiferromagnetism in Ru2MnZ (Z=Sn, Sb, Ge, Si) full Heusler alloys: Effects of magnetic frustration and chemical disorder, Phys. Rev. B - Condens. Matter Mater. Phys. **91**, 094432 (2015), arXiv:1501.05116 .
